# Supplementary material for: Measurement of inclusive and differential cross sections in the $H \rightarrow ZZ^* \rightarrow 4\ell$ decay channel in $pp$ collisions at $\sqrt{s}$ = 13 TeV with the ATLAS detector
Source: arXiv:1708.02810 source file (2018-02-20)
Supplement: Supplementary file 1 [file Appendix.tex]

\label{appendix}

- additional unfolded plots:  \monetwo, \detajj: Figure~\ref{fig:app_xs_extra}, \nbjets: Figure~\ref{fig:app_xs_bjets} \\
- CR plots for \ptfourl\ and \njets: Figure~\ref{fig:app_cr}\\
- reco level plots for all variables: Figure~\ref{fig:app_reco}\\
- correction factor plots for all variables: Figure~\ref{fig:app_corrfactors} \\
- table of used binnings: Table~\ref{tab:app_bin1} and~\ref{tab:app_bin2} \\
- table of measured XS: Table~\ref{tab:app_XS}\\
- table of correction factors: Table~\ref{tab:app_CF}\\

\begin{figure}[!htbp]
\centering
\subfigure[\label{fig:m12}]{\includegraphics[width=0.45\linewidth]{fit_m12_N3LO_data_unfolded.pdf}}
\subfigure[\label{fig:etajj}]{\includegraphics[width=0.45\linewidth]{fit_etajj_N3LO_data_unfolded.pdf}}
\caption{Additional fiducial differential cross sections for (a) the invariant mass of the leading lepton pair \monetwo, and (b) the angle between the two leading jets \detajj. The measured distributions are compared to ggF predictions by \progname{NNLOPS} and \mgfxfx, all normalized to the N3LO cross section. Predictions for all other Higgs production modes $XH$ are added. The error bars on the data points show the total uncertainties, while the systematic uncertainties are indicated by the boxes. The shaded bands on the expected cross sections indicate the PDF and scale uncertainties. The $p$-values indicating the compatibility of the measurement and the SM prediction are shown as well. They do not include the systematic uncertainty in the theoretical predictions.
\label{fig:app_xs_extra}}
\end{figure}

\begin{figure}[!htbp]
\centering
\includegraphics[width=0.45\linewidth]{fit_nbjet_N3LO_data_unfolded.pdf}
\caption{Distribution of the number of $b$-jets in \hfourl\ events. The $b$-jets are reconstructed using flavour-tagging with the MV2c10 algorithm at 70\% efficiency [ATL-PHYS-PUB-2016-012], with the corresponding uncertainties taken into account. At particle-level, each jet is labeled as a $b$-jet if there is at least one electroweakly decaying $B$-hadron ghost-associated to it. The measured distributions are compared to ggF predictions by \progname{NNLOPS}  and \mgfxfx, all normalized to the N3LO cross section. Predictions for all other Higgs production modes $XH$ are added. The error bars on the data points show the total uncertainties, while the systematic uncertainties are indicated by the boxes. The shaded bands on the expected cross sections indicate the PDF and scale uncertainties. The $p$-values indicating the compatibility of the measurement and the SM prediction are shown as well. They do not include the systematic uncertainty in the theoretical predictions.
\label{fig:app_xs_bjets}}
\end{figure}

\begin{figure}[!htbp]
\centering
\subfigure[\label{fig:cr_pt_llmumu}]{\includegraphics[width=0.4\linewidth]{plot_h_pt_all_binned_mu_all.pdf}}
\subfigure[\label{fig:cr_njet_llmumu}]{\includegraphics[width=0.4\linewidth]{plot_h_njets_binned_mu_all.pdf}}
\caption{
Control region plots for (a) \ptH\ and (b) \njets.
The event selection is modified by relaxing the isolation requirements on the second dimuon pair.
\label{fig:app_cr}}
\end{figure}

\begin{figure}[!htbp]
\centering
\subfigure[\label{fig:r_y}]{\includegraphics[width=0.3\linewidth]{hy_incl_Data.pdf}}
\subfigure[\label{fig:r_cts}]{\includegraphics[width=0.3\linewidth]{hcts_incl_Data.pdf}}
\subfigure[\label{fig:r_cts}]{\includegraphics[width=0.3\linewidth]{hljpt_incl_Data.pdf}}
\subfigure[\label{fig:r_phijj}]{\includegraphics[width=0.3\linewidth]{hphijj_incl_Data.pdf}}
\subfigure[\label{fig:r_mjj}]{\includegraphics[width=0.3\linewidth]{hmjjrm_incl_Data.pdf}}
\subfigure[\label{fig:r_pt0j}]{\includegraphics[width=0.3\linewidth]{hpt0j_incl_Data_log.pdf}}
\subfigure[\label{fig:r_pt1j}]{\includegraphics[width=0.3\linewidth]{hpt1j_incl_Data_log.pdf}}
\subfigure[\label{fig:r_pt2j}]{\includegraphics[width=0.3\linewidth]{hpt2j_incl_Data_log.pdf}}
\caption{Reconstructed event yields for different observables. The error bars on the data points indicate the statistical uncertainty. The  uncertainty in the prediction is shown by the dashed band. \label{fig:app_reco}}
\end{figure}

\begin{figure}[!htbp]
\centering
\subfigure[\label{fig:r_m12}]{\includegraphics[width=0.3\linewidth]{hm12_incl_Data.pdf}}
\subfigure[\label{fig:r_etajj}]{\includegraphics[width=0.3\linewidth]{hetajj_incl_Data.pdf}}
\subfigure[\label{fig:r_nbjet}]{\includegraphics[width=0.3\linewidth]{hnbjet_incl_Data.pdf}}
\caption{Reconstructed event yields for different observables. The error bars on the data points indicate the statistical uncertainty. The  uncertainty in the prediction is shown by the dashed band. \label{fig:app_reco_add}}
\end{figure}

\begin{figure}[!htbp]
\centering
\subfigure[\label{fig:c_y}]{\includegraphics[width=0.3\linewidth]{HZZ_13TeV_purity_and_C_y_nominal_production}}
\subfigure[\label{fig:c_cthstr}]{\includegraphics[width=0.3\linewidth]{HZZ_13TeV_purity_and_C_cthstr_nominal_production}}
\subfigure[\label{fig:c_m34}]{\includegraphics[width=0.3\linewidth]{HZZ_13TeV_purity_and_C_m34_nominal_production}}
\subfigure[\label{fig:c_j1pt}]{\includegraphics[width=0.3\linewidth]{HZZ_13TeV_purity_and_C_j1pt_nominal_production}}
\subfigure[\label{fig:c_jj_m}]{\includegraphics[width=0.3\linewidth]{HZZ_13TeV_purity_and_C_jj_m_nominal_production}}
\subfigure[\label{fig:c_jj_phi}]{\includegraphics[width=0.3\linewidth]{HZZ_13TeV_purity_and_C_jj_phi_nominal_production}}
\subfigure[\label{fig:c_pt_0jet}]{\includegraphics[width=0.3\linewidth]{HZZ_13TeV_purity_and_C_pt_0jet_nominal_production}}
\subfigure[\label{fig:c_pt_1jet}]{\includegraphics[width=0.3\linewidth]{HZZ_13TeV_purity_and_C_pt_1jet_nominal_production}}
\subfigure[\label{fig:c_pt_2jet}]{\includegraphics[width=0.3\linewidth]{HZZ_13TeV_purity_and_C_pt_2jet_nominal_production}}
\subfigure[\label{fig:c_m12m34}]{\includegraphics[width=0.3\linewidth]{HZZ_13TeV_purity_and_C_m12m34_nominal_production}}
\caption{Bin-by-bin correction factors and bin purities. The bands show the systematic uncertainties in the correction factors, which are discussed in Section~\ref{sec:systematics}.
 The uncertainties in the bin purity include the detector response and pile-up uncertainties. \label{fig:app_corrfactors}}
\end{figure}

\begin{figure}[!htbp]
\centering
\subfigure[\label{fig:c_m12}]{\includegraphics[width=0.3\linewidth]{HZZ_13TeV_purity_and_C_m12_nominal_production}}
\subfigure[\label{fig:c_jj_eta}]{\includegraphics[width=0.3\linewidth]{HZZ_13TeV_purity_and_C_jj_eta_nominal_production}}
\subfigure[\label{fig:c_nbjets}]{\includegraphics[width=0.3\linewidth]{HZZ_13TeV_purity_and_C_nbjets_nominal_production}}
\caption{Bin-by-bin correction factors and bin purities. The bands show the systematic uncertainties in the correction factors, which are discussed in Section~\ref{sec:systematics}.
 The uncertainties in the bin purity include the detector response and pile-up uncertainties. \label{fig:app_corrfactors_add}}
\end{figure}

\begin{table}
\centering
\caption{Bin boundaries and number of bins of the differential distributions.\label{tab:app_bin1} }
\vspace{0.2cm}
\begin{tabular}{lll}
  \hline\hline
  Variable & Bin boundaries & $N_{\mathrm{bins}}$\\
  \hline
  $p_{T}$ & 0, 10, 15, 20, 30, 45, 60, 80, 120, 200, 350 GeV
  & 10 \\
  $p_{T}^{N_{\mathrm{jets}}=0}$ & 0, 15, 30, 120, 350 GeV     & 4\\
  $p_{T}^{N_{\mathrm{jets}}=1}$ & 0, 30, 60, 80, 120, 350 GeV & 5\\
  $p_{T}^{N_{\mathrm{jets}}\geq2}$ & 0, 120, 350 GeV          & 2\\

  $|cos(\theta^{*})|$ & 0, 0.125, 0.25, 0.375, 0.5, 0.625, 0.75, 0.875, 1.0
  & 8 \\
  $m_{34}$ & 12, 20, 24, 28, 32, 40, 55, 65 GeV & 7 \\
  $N_{\mathrm{jets}}$ & 0, 1, 2, $\geq$1, $\geq$2, $\geq$3 & 6\\
  $p_{T}^{\mathrm{lead.\;jet}}$ & 30, 40, 55, 75, 120, 350
  GeV & 5 \\
  \mjj & 0, 120, 3000 GeV & 2 \\
  \dphijj & 0, $\pi$, 2$\pi$ & 2\\
  $m_{12}$ & 50, 65, 74, 82, 88, 94, 106 GeV & 6 \\
  \detajj & 0, 2, 10 & 2 \\
  $N_{b-\mathrm{jets}}$ & 0,  $\geq$1 & 2 \\
  \hline\hline
\end{tabular}
\end{table}

\begin{table}
\centering
\caption{Bin boundaries of the \monetwo\ vs \mthreefour\ distribution. \label{tab:app_bin2} }
\vspace{0.2cm}
\begin{tabular}{lll}
  \hline\hline
  Bin & $m_{12}$ and $m_{34}$ values [GeV] \\
  \hline
  0 & $m_{12}<82$ and $m_{34}<32$ \\
  1 & $m_{12}<74$ and $m_{34}>32$ \\
  2 & $m_{12}>74$ and $m_{34}>32$ \\
  3 & $m_{12}>82$ and $24<m_{34}<32$ \\
  4 & $m_{12}>82$ and $m_{34}<24$ \\
  \hline\hline
\end{tabular}
\end{table}

\begin{sidewaystable}
\centering
\tiny
\caption{Measured differential cross sections in bins of the observables of interest, divided by the bin width. \label{tab:app_XS} }
\vspace{0.2cm}
\begin{tabular}{ lcccccccccc }
\hline
\hline
 & Bin 1 & Bin 2 & Bin 3 & Bin 4 & Bin 5 & Bin 6 & Bin 7 & Bin 8 & Bin 9 & Bin 10 \\
\hline
d$\sigma$/d\ptH  & $0.070^{+0.027}_{-0.023}$ & $0.018^{+0.027}_{-0.020}$ & $0.072^{+0.037}_{-0.030}$ & $0.042^{+0.021}_{-0.017}$ & $0.034^{+0.014}_{-0.012}$ & $0.0169^{+0.010}_{-0.008}$ & $0.0108^{+0.0074}_{-0.0056}$ & $0.0137^{+0.0050}_{-0.0041}$ & $0.0043^{+0.0020}_{-0.0015}$ & $0.00118^{+0.00072}_{-0.00051}$ \\

d$\sigma$/d\yH & $2.13^{+0.78}_{-0.65}$ & $2.42^{+0.83}_{-0.70}$ & $1.63^{+0.69}_{-0.58}$ & $2.14^{+0.79}_{-0.67}$ & $1.50^{+0.59}_{-0.50}$ & $1.35^{+0.56}_{-0.45}$ & $0.18^{+0.23}_{-0.14}$ & - & - & - \\

d$\sigma$/d\costhetastar & $3.8^{+1.6}_{-1.4}$ & $4.1^{+1.7}_{-1.4}$ & $4.6^{+1.8}_{-1.5}$ & $4.8^{+1.8}_{-1.5}$ & $1.2^{+1.2}_{-0.8}$ & $3.5^{+1.6}_{-1.3}$ & $4.2^{+1.7}_{-1.4}$ & $3.3^{+1.6}_{-1.3}$ & - & -  \\

d$\sigma$/d\mthreefour & $0.064^{+0.034}_{-0.030}$ & $0.153^{+0.061}_{-0.050}$ & $0.216^{+0.065}_{-0.056}$ & $0.176^{+0.060}_{-0.051}$ & $0.061^{+0.025}_{-0.021}$ & $0.0345^{+0.013}_{-0.010}$  & 95\% C.L. limit & - & - & - \\

$\sigma$ (\monetwo vs \mthreefour) & $0.46^{+0.19}_{-0.16}$ & $0.51^{+0.19}_{-0.16}$ & $0.48^{+0.20}_{-0.17}$ & $1.35^{+0.33}_{-0.29}$ & $0.85^{+0.34}_{-0.30}$ & - & - & - & - & -  \\

$\sigma$ (\njets) &  $1.74^{+0.47}_{-0.41}$ & $0.99^{+0.28}_{-0.24}$ & $0.54^{+0.20}_{-0.16}$ & $1.88^{+0.40}_{-0.35}$ & $0.87^{+0.27}_{-0.22}$ & 
$0.32^{+0.17}_{-0.12}$ & - & - & - & - \\

d$\sigma$/d\jetpt & $0.0371^{+0.017}_{-0.014}$ & $0.020^{+0.011}_{-0.008}$ & $0.0141^{+0.0075}_{-0.0058}$ & $0.0102^{+0.0041}_{-0.0033}$ & $0.00205^{+0.00079}_{-0.00063}$ & - & - & - & - & - \\

d$\sigma$/d\dphijj & $0.167^{+0.062}_{-0.059}$ & $0.107^{+0.051}_{-0.040}$ & - & - & - & - & - & - & - & - \\

d$\sigma$/d\mjj & $0.00074^{+0.00077}_{-0.00051}$ & $0.000276^{+0.000085}_{-0.000069}$ & - & - & - & - & - & - & - & - \\

d$\sigma$ /d\ptH\ (0j) & $0.0431^{+0.019}_{-0.016}$ & $0.032^{+0.017}_{-0.014}$ & $0.0067^{+0.0028}_{-0.0022}$  & 95\% C.L. limit & - & - & - & - & - & - \\

d$\sigma$ /d\ptH\ (1j) & $0.0075^{+0.0040}_{-0.0029}$ & $0.0024^{+0.0037}_{-0.0024}$ & $0.0084^{+0.0068}_{-0.0048}$ & $0.0078^{+0.0040}_{-0.0030}$ & $0.00060^{+0.00047}_{-0.00032}$ & - & - & - & - & - \\

d$\sigma$ /d\ptH ($\ge$2j) & $0.0041^{+0.0017}_{-0.0013}$ & $0.00162^{+0.00068}_{-0.00054}$  & - & - & - & - & - & - & - & - \\
d$\sigma$/d\monetwo & $0.022^{+0.011}_{-0.008}$ & $0.032^{+0.017}_{-0.014}$ & $0.077^{+0.026}_{-0.022}$ & $0.095^{+0.031}_{-0.027}$ & $0.314^{+0.080}_{-0.072}$ & $0.0000^{+0.0054}_{-0.0036}$ & - & - & - & - \\

d$\sigma$/d\detajj & $0.175^{+0.086}_{-0.066}$ & $0.071^{+0.026}_{-0.021}$ & - & - & - & - & - & - & - & -  \\

d$\sigma$/d\nbjets & $3.49^{+0.57}_{-0.53}$ & $0.17^{+0.14}_{-0.09}$ & - & - & - & - & - & - & - & -  \\
\hline
\hline
\end{tabular}
\end{sidewaystable}

%new table

\begin{sidewaystable}
\centering
\caption{Correction factors as a function of the different observables. The shown uncertainties are the total uncertainties discussed in Section~\ref{sec:systematics}. \label{tab:app_CF} }
\vspace{0.2cm}
\begin{tabular}{ lcccccccccc }
\hline
\hline
 & Bin 1 & Bin 2 & Bin 3 & Bin 4 & Bin 5 & Bin 6 & Bin 7 & Bin 8 & Bin 9 & Bin 10 \\
\hline
incl & 53.3 $\pm$ 3.1 & - & - & - & - & - & - & - & - & -\\

\ptH  & 53.6 $\substack{+3.1 \\ -3.0}$ & 53.2 $\substack{+3.2 \\ -3.0}$ & 52.9 $\pm$ 3.0 & 52.7 $\substack{+3.1 \\ -3.0}$ & 52.3 $\pm$ 3.1 & 51.9 $\pm$ 3.2 & 52.4 $\substack{+3.6 \\ -3.5}$  & 53.9 $\pm$ 3.9 & 56.9 $\pm$ 4.4  & 61.1 $\pm$ 5.7 \\

\ptH\ (0j) & 50.0 $\substack{+3.6 \\ -3.4}$ & 48.1 $\substack{+4.5 \\ -4.4}$  & 48.4 $\substack{+9.1 \\ -8.9}$  & 58.2 $\substack{+7.7 \\ -7.5}$  & - & - & - & - & - & - \\

\ptH\ (1j) & 99 $\substack{+14 \\ -13}$ & 52.6 $\substack{+4.7 \\ -4.8}$  & 47.7 $\substack{+3.8 \\ -3.9}$ & 49.6 $\substack{+5.9 \\ -6.0}$ & 53.7 $\substack{+6.3 \\ -6.6}$ & - & - & - & - & - \\

\ptH ($\ge$2j) &  64 $\pm$ 15 & 59.9 $\pm$ 7.1 & - & - & - & - \\

\yH & 54.5 $\pm$ 3.1 & 54.1 $\pm$ 3.1 & 54.0 $\pm$ 3.1 & 54.3 $\substack{+3.2 \\ -3.1}$  & 52.2 $\substack{+3.2 \\ -3.1}$ & 50.0 $\pm$ 3.1 & 43.3 $\pm$ 3.2  & - & - & - \\

\costhetastar & 53.8 $\pm$ 3.1 & 53.8 $\substack{+3.2 \\ -3.1}$  & 54.0 $\pm$ 3.2 & 53.5 $\substack{+3.1 \\ -3.0}$ & 53.3 $\pm$ 3.1 & 52.8 $\pm$ 3.0 & 52.7 $\substack{+3.1 \\ -3.0}$ & 52.3 $\pm$ 3.3  & - & -  \\

\mthreefour & 53.6 $\substack{+3.2 \\ -3.1}$ & 53.8 $\substack{+3.3 \\ -3.2}$ & 53.7 $\substack{+3.2 \\ -3.1}$ & 51.2 $\pm$ 3.2 & 53.0 $\pm$ 3.2 & 56.3 $\substack{+3.1 \\ -3.0}$  & 52.2 $\substack{+3.2 \\ -3.1}$ & - & - & - \\

\monetwo\ vs \mthreefour & 62.4 $\pm$ 3.4 & 58.3 $\substack{+3.1 \\ -3.0}$ & 50.8 $\pm$ 3.3 & 51.1 $\pm$ 3.1 & 52.6 $\pm$ 3.2  & - & - & - & - & -  \\

\njets &  48.9 $\substack{+5.0 \\ -4.8}$ & 56.1 $\substack{+3.7 \\ -3.6}$ & 60.9 $\substack{+6.6 \\ -6.7}$ & 58.6 $\substack{+6.5 \\ -6.3}$   & 63 $\pm$ 12 &   67 $\substack{+28 \\ -27}$  & - & - & - & - \\

\jetpt & 65.2 $\substack{+7.0 \\ -6.6}$ & 56.2 $\substack{+5.5 \\ -5.3}$ & 56.0 $\substack{+5.5 \\ -5.3}$ & 56.9 $\pm$ 6.1 & 58.1 $\substack{+8.5 \\ -8.4}$ & - & - & - & - & - \\

\mjj & 65 $\pm$ 13 & 61 $\pm$ 12 & - & - & - & - & - & - & - & - \\

\dphijj & 63 $\pm$ 12 & 62 $\pm$ 13 & - & - & - & - & - & - & - & - \\

$m_{12}$  & 59.6 $\pm$ 3.2 & 57.7 $\substack{+3.2 \\ -3.1}$ & 60.0 $\substack{+3.2 \\ -3.1}$  & 76.7 $\substack{+3.3 \\ -3.2}$  & 42.7 $\pm$ 3.3  & 91.2 $\substack{+5.6 \\ -5.7}$ & - & - & - & -\\

\detajj & 60 $\pm$ 15 & 65.4 $\substack{+9.6 \\ -9.2}$ & - & - & - & - & - & - & - & -  \\

\nbjets &  53.6 $\substack{+3.1 \\ -3.1}$ & 44 $\pm$ 36 & - & - & - & - & - & - & - & -  \\
\hline
\hline
\end{tabular}
\end{sidewaystable}
